# Supplementary material for: Scene Style Text Editing
Source: arXiv:2304.10097 source file (2023-04-20)
Supplement: Supplementary file 1 [file 7-Appendix.tex]

\appendix

\section{Code Details} \label{code_detail}
Our QuadNet model consists of four parts, that is, background inpainting, style encoder, content encoder and fusion generator. 
Our implementation has been developed with the help of many canonical open-sourced projects, including ResNet \cite{He_2016_CVPR}, VGGNet \cite{simonyan2014very}, StyleGAN \cite{karras2019style}, LaMa \cite{suvorov2022resolution}, Recognizer \cite{baek2019wrong}, etc.
Here we show the structure and code of some core components. 
Figure \ref{fig.mappingnet} shows the structure of StyleMapNet, which employs a 3-layer MLP with LeakyReLU activation function. 
Its input is a 512-dimensional style vector $\mathbf{z}$, and output is a $2 \times 512 \times 5$-dimensional vector.
Then the 5120D vector is divided into 5 latent style vectors, and Figure \ref{fig.apply_style} shows how to use AdaIN to inject each latent vector into the feature map x. 
In addition, we also used other open source methods for comparison, including SeFa \cite{shen2021closed}, SRNet \cite{wu2019editing} and Palette \cite{saharia2022palette}.
The open-source SeFa code can only handle images with the same height and width, we made some changes to make it able to edit images with shape [64, 256].
Since the original SRNet paper has no open code, a third-party reproduction of the code was used.
Palette is a diffusion model \cite{nichol2021improved}, which was originally used to deal with image restoration, colorization and other issues. 
We concatenate $I_s$ and $T_{c2}$ along the channel axis as a condition to guide the generation of the diffusion model.
All codes will be open upon acceptance.

\section{Dataset Details}
In the experiments we adopted synthetic and real-world data.
The synthetic data structure method is similar to that of SRNet \cite{wu2019editing}. 
It is mainly synthesized based on some open source data, including text-free background images provided by SynthText \cite{Gupta16}, some open source font files searched from the Internet, and an English vocabulary.
All related material will be released upon acceptance.

The real-world data is from diverse sources, including SROIE, COCO ~\cite{veit2016coco}, ReCTS, ArT, LSVT, ICDAR2015 ~\cite{karatzas2015icdar}, MLT2019 ~\cite{nayef2019icdar2019}, ICDAR2019.
The training set consists of a total of 33,207 images and the test set contains 1,000 images.
The sources focuse on the detection and recognition in real-world, with detailed text box annotations and text content labels.
We first cut out the style picture ${I}_s$ on original image according to the text box annotation, then enlarge the text box size and then crop to obtain the large style image $I_{Ls}$. 
$I_{Ms}$ is a binary image, and the white part marks the text position.
We discard lowresolution image $I_{s}$ with a height of less than 32 pixels. 

We will provide a list of real-world dataset after the paper is accepted.
Figure \ref{fig.data_label} shows one of the list, which describes the information of Figure \ref{fig.data_real} (appears as Figure 5 in the main body of the paper), including text content (``Row"), new target text (``boob"), and which dataset the image comes from (``datasets/Art/detection/train\_images/gt\_3992.jpg").

\begin{figure}[t]
\centering 
\includegraphics[width=0.42\textwidth]{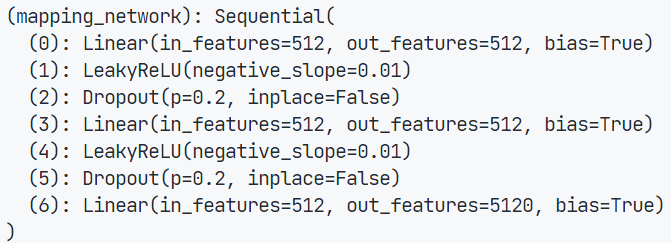}
\caption{The structure of StyleMapNet.}
\label{fig.mappingnet}
\end{figure}

\begin{figure}[t]
\centering 
\includegraphics[width=0.42\textwidth]{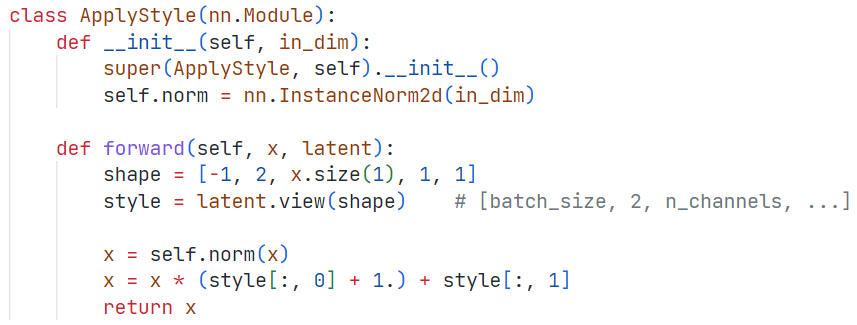}
\caption{Use AdaIN to inject the latent style vector into the feature map x.}
\label{fig.apply_style}
\end{figure}
\input{figures/combination/data_real.tex}

\begin{figure}[t]
\centering 
\includegraphics[width=0.42\textwidth]{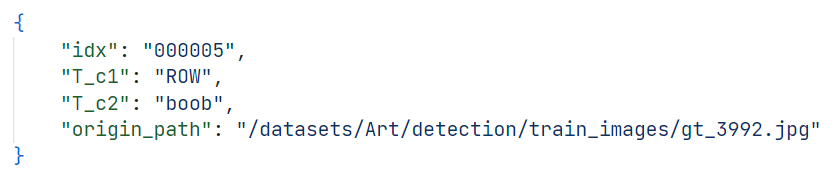}
\caption{Text annotation of a real-world Figure \ref{fig.data_real}.}
\label{fig.data_label}
\end{figure}

\input{figures/combination/W_t-SNE.tex}
\begin{figure*}[t]
\centering 
\subfigure[$\mathbf {z}$ about rotate]{
\label{Fig.z.rotate}
\includegraphics[width=0.3\textwidth, trim=30 10 0 50]{figures/tsne/z/style_vector_rotate.png}}
\subfigure[$\mathbf {z}$ about font]{
\label{Fig.z.font}
\includegraphics[width=0.3\textwidth, trim=30 10 0 50]{figures/tsne/z/style_vector_font.png}}
\subfigure[$\mathbf {z}$ about color]{
\label{Fig.z.color}
\includegraphics[width=0.3\textwidth, trim=30 10 0 50]{figures/tsne/z/style_vector_color.png}}
\caption{t-SNE visualizations of $\mathbf{z}$ about text style attributes: 
corresponding to the three images in Figure \ref{fig.W_t-SNE}, $\mathbf {z}$ is not as distinguishable as the $\mathbf{w}^{i}$ with regard to attributes such as rotation angle, font, and color.}
\label{fig.z_t-SNE}
\end{figure*}

\begin{figure}[t]
\centering 
\includegraphics[width=0.42\textwidth]{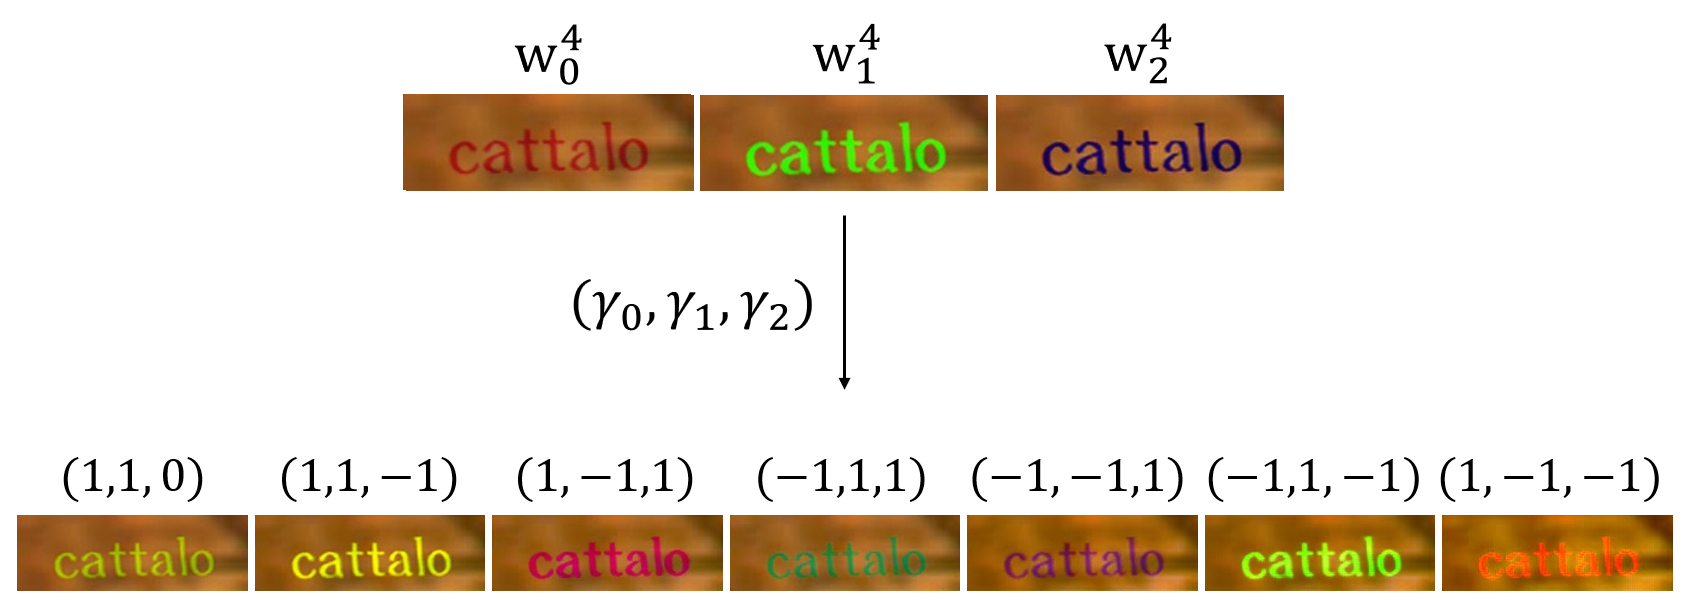}
\caption{Linearly interpolating two latent codes. Combine red, green and blue vector to get other colors: $\mathbf{w}^{4}_{0}$, $\mathbf{w}^{4}_{1}$ and $\mathbf{w}^{4}_{2}$ represent red, green and blue, $({\gamma}_{0}, {\gamma}_{1}, {\gamma}_{2})=(1,1,0),\ldots, (1,-1,-1)$, $\mathbf{w}^{4} = 0.5 \times ({\gamma}_{0} \mathbf{w}^{4}_{0} + {\gamma}_{1} \mathbf{w}^{4}_{1} + {\gamma}_{2} \mathbf{w}^{4}_{2}$).}
\label{fig.interpolation}
\end{figure}

\begin{figure*}[t]
\centering
\begin{minipage}{0.16\linewidth}
\centering
    Source Image
	\includegraphics[width=1\linewidth, height=0.4\linewidth]{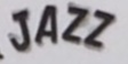}
\end{minipage}
\begin{minipage}{0.16\linewidth}
	\centering
    New Content
	\includegraphics[width=1\linewidth, height=0.4\linewidth]{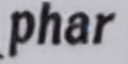}
\end{minipage}
\begin{minipage}{0.16\linewidth}
	\centering
 Source Image
	\includegraphics[width=1\linewidth, height=0.4\linewidth]{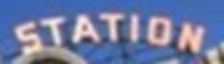}
\end{minipage}
\begin{minipage}{0.16\linewidth}
	\centering
 New Content
	\includegraphics[width=1\linewidth, height=0.4\linewidth]{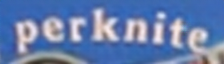}
\end{minipage}
\begin{minipage}{0.16\linewidth}
	\centering
 Source Image
	\includegraphics[width=1\linewidth, height=0.4\linewidth]{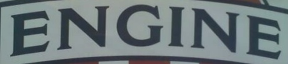}
\end{minipage}
\begin{minipage}{0.16\linewidth}
    \centering
    New Content
    \includegraphics[width=1\linewidth, height=0.4\linewidth]{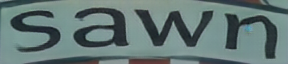}
\end{minipage}

\begin{minipage}{0.16\linewidth}
	\centering
	\includegraphics[width=1\linewidth, height=0.4\linewidth]{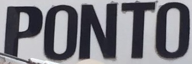}
\end{minipage}
\begin{minipage}{0.16\linewidth}
	\centering
	\includegraphics[width=1\linewidth, height=0.4\linewidth]{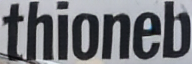}
\end{minipage}
\begin{minipage}{0.16\linewidth}
	\centering
	\includegraphics[width=1\linewidth, height=0.4\linewidth]{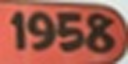}
\end{minipage}
\begin{minipage}{0.16\linewidth}
	\centering
	\includegraphics[width=1\linewidth, height=0.4\linewidth]{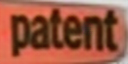}
\end{minipage}
\begin{minipage}{0.16\linewidth}
	\centering
	\includegraphics[width=1\linewidth, height=0.4\linewidth]{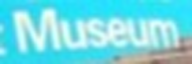}
\end{minipage}
\begin{minipage}{0.16\linewidth}
    \centering
    \includegraphics[width=1\linewidth, height=0.4\linewidth]{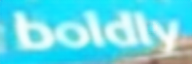}
\end{minipage}

\begin{minipage}{0.16\linewidth}
	\centering
	\includegraphics[width=1\linewidth, height=0.4\linewidth]{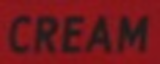}
\end{minipage}
\begin{minipage}{0.16\linewidth}
	\centering
	\includegraphics[width=1\linewidth, height=0.4\linewidth]{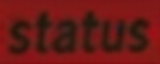}
\end{minipage}
\begin{minipage}{0.16\linewidth}
	\centering
	\includegraphics[width=1\linewidth, height=0.4\linewidth]{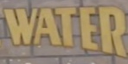}
\end{minipage}
\begin{minipage}{0.16\linewidth}
	\centering
	\includegraphics[width=1\linewidth, height=0.4\linewidth]{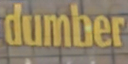}
\end{minipage}
\begin{minipage}{0.16\linewidth}
	\centering
	\includegraphics[width=1\linewidth, height=0.4\linewidth]{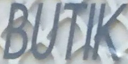}
\end{minipage}
\begin{minipage}{0.16\linewidth}
    \centering
    \includegraphics[width=1\linewidth, height=0.4\linewidth]{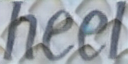}
\end{minipage}

\begin{minipage}{0.16\linewidth}
	\centering
	\includegraphics[width=1\linewidth, height=0.4\linewidth]{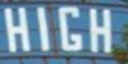}
\end{minipage}
\begin{minipage}{0.16\linewidth}
	\centering
	\includegraphics[width=1\linewidth, height=0.4\linewidth]{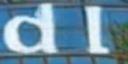}
\end{minipage}
\begin{minipage}{0.16\linewidth}
	\centering
	\includegraphics[width=1\linewidth, height=0.4\linewidth]{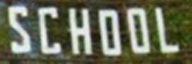}
\end{minipage}
\begin{minipage}{0.16\linewidth}
	\centering
	\includegraphics[width=1\linewidth, height=0.4\linewidth]{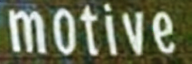}
\end{minipage}
\begin{minipage}{0.16\linewidth}
	\centering
	\includegraphics[width=1\linewidth, height=0.4\linewidth]{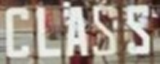}
\end{minipage}
\begin{minipage}{0.16\linewidth}
    \centering
    \includegraphics[width=1\linewidth, height=0.4\linewidth]{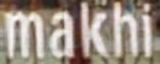}
\end{minipage}

\begin{minipage}{0.16\linewidth}
	\centering
	\includegraphics[width=1\linewidth, height=0.4\linewidth]{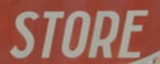}
\end{minipage}
\begin{minipage}{0.16\linewidth}
	\centering
	\includegraphics[width=1\linewidth, height=0.4\linewidth]{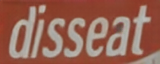}
\end{minipage}
\begin{minipage}{0.16\linewidth}
	\centering
	\includegraphics[width=1\linewidth, height=0.4\linewidth]{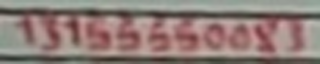}
\end{minipage}
\begin{minipage}{0.16\linewidth}
	\centering
	\includegraphics[width=1\linewidth, height=0.4\linewidth]{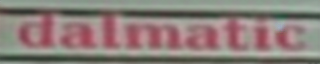}
\end{minipage}
\begin{minipage}{0.16\linewidth}
	\centering
	\includegraphics[width=1\linewidth, height=0.4\linewidth]{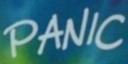}
\end{minipage}
\begin{minipage}{0.16\linewidth}
    \centering
    \includegraphics[width=1\linewidth, height=0.4\linewidth]{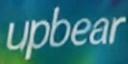}
\end{minipage}

\begin{minipage}{0.16\linewidth}
	\centering
	\includegraphics[width=1\linewidth, height=0.4\linewidth]{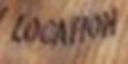}
\end{minipage}
\begin{minipage}{0.16\linewidth}
	\centering
	\includegraphics[width=1\linewidth, height=0.4\linewidth]{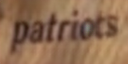}
\end{minipage}
\begin{minipage}{0.16\linewidth}
	\centering
	\includegraphics[width=1\linewidth, height=0.4\linewidth]{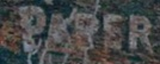}
\end{minipage}
\begin{minipage}{0.16\linewidth}
	\centering
	\includegraphics[width=1\linewidth, height=0.4\linewidth]{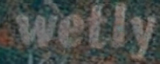}
\end{minipage}
\begin{minipage}{0.16\linewidth}
	\centering
	\includegraphics[width=1\linewidth, height=0.4\linewidth]{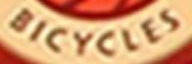}
\end{minipage}
\begin{minipage}{0.16\linewidth}
    \centering
    \includegraphics[width=1\linewidth, height=0.4\linewidth]{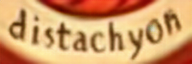}
\end{minipage}

\begin{minipage}{0.16\linewidth}
	\centering
	\includegraphics[width=1\linewidth, height=0.4\linewidth]{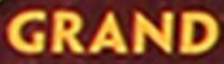}
\end{minipage}
\begin{minipage}{0.16\linewidth}
	\centering
	\includegraphics[width=1\linewidth, height=0.4\linewidth]{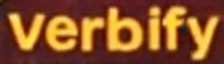}
\end{minipage}
\begin{minipage}{0.16\linewidth}
	\centering
	\includegraphics[width=1\linewidth, height=0.4\linewidth]{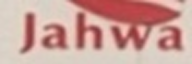}
\end{minipage}
\begin{minipage}{0.16\linewidth}
	\centering
	\includegraphics[width=1\linewidth, height=0.4\linewidth]{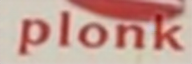}
\end{minipage}
\begin{minipage}{0.16\linewidth}
	\centering
	\includegraphics[width=1\linewidth, height=0.4\linewidth]{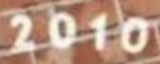}
\end{minipage}
\begin{minipage}{0.16\linewidth}
    \centering
    \includegraphics[width=1\linewidth, height=0.4\linewidth]{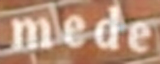}
\end{minipage}

\caption{Generated images by our QuadNet with new content: change the text content and keep the text style and background texture of the source image, which are drawn from real-world data.
}
\label{fig:real_scene}
\end{figure*}

\section{Evaluation Metrics}
We adopt several quantitative evaluation metrics that are commonly used in image generation, and the codes for measuring these metrics are included in the code of Section \ref{code_detail}.
The metrics includes:
1) Frechet Inceptionthe distance (FID) ~\cite{NIPS2017_8a1d6947}: evaluates the distance between two image distributions and can be used as a reference for the consistency of the style between the generated images and the source images; 
2) Learned Perceptual Image Patch Similarity (LPIPS) ~\cite{zhang2018unreasonable}: measures the perceptual similarity between two images.
We calculate the similarity between each generated image and its corresponding ground truth in the test set and obtain the average similarity;
3) text recognition accuracy: using a text recognition engine ~\cite{baek2019wrong}, tests whether the content generated in the image is correct, and is considered correct only if the recognition result is exactly the same as the label. 
It is computed as: 
\begin{equation}
accuracy=\frac{1}{ N_{test} } \left(\sum_{i} \mathbb{I}\left(\mathbf{R}(G_{c2_{i}})==S_{c2_{i}}\right)\right).
\end{equation}

\section{Extended Investigation of Latent Space Editing}
This section is an extension of Section 4.2 of the main body of the paper. 
First, we compared the t-SNE ~\cite{van2008visualizing} visualization results of the $\mathbf{z}$ and $\mathbf{w}^{i}$ vectors, indicating that the $\mathbf{z}$ vector does not decouple the text style well, while the $\mathbf{w}^{i}$ vectors obtained after StyleMapNet successfully separates the text style into attributes of rotation angle, font, and color. 
Then, we further explored whether the additive color theory in the color latent space we constructed are consistent with reality.

The visualization results of t-SNE are shown in Figure \ref{fig.W_t-SNE} and Figure \ref{fig.z_t-SNE}, in which the same color represents the same attribute. 
In Figure \ref{fig.W_t-SNE} (a), the image vectors $\mathbf{w}^{0}$ corresponding to the 5 text rotation angles are well distinguished, and the ${0}^{\circ}$ and ${5}^{\circ}$, ${-5}^{\circ}$ vectors are relatively close to each other, the ${15}^{\circ}$ and ${-15}^{\circ}$ vectors are relatively far apart.
Figure \ref{fig.W_t-SNE} (b) shows that layer vector $\mathbf{w}^{123}$ affect the font, the $\mathbf{w}^{123}$ vector corresponding to different fonts are well separated.
Similarly, Figure \ref{fig.W_t-SNE} (c) shows that layer vector $\mathbf{w}^{4}$ dominates on the color. 
As a contrast, style vector $\mathbf{z}$ is not suitable to distinguish rotation angle, font or color well, as shown in Figure \ref{fig.z_t-SNE} (a), \ref{fig.z_t-SNE} (b) and \ref{fig.z_t-SNE} (c). 
Therefore, our semantic editing in latent space uses $\mathbf{w}^{i}$ instead of $\mathbf{z}$.

Additionally, we observed an interesting phenomenon where the color mixing in the two-dimensional color space is somewhat consistent with that in the real world, as shown in Figure \ref{fig.W_t-SNE} (c).
Specifically, we all know that the rules of color mixing are as follows:
red + green = yellow, blue + green = cyan, and red + blue = purple, so does the color distribution of Figure \ref{fig.W_t-SNE} (c), which reduces the vector $\mathbf{w}^{4}$ to a two-dimensional space, match this pattern?
First we calculate to obtain these color mean centroids, such as red (27.09, -38.42), green (-43.38, -8.06), blue (43.79, 41.83), yellow (-23.89, -35.99), cyan (-51.71, 26.81), and purple (29.82, 17.39).
Then binary quadratic equations based on the color summation rule give the following color mixing formula: 0.726 red + 1.004 green = yellow, 1.081 blue + 2.283 green = cyan, 0.173 red + 0.574 blue = purple, which is somewhat similar to that in the real world.
Moreover, we mix $\mathbf{w}^{4}$ vectors in higher dimensional space, and try color mixing to tune out other colors from red, green and blue.
As shown in the Figure \ref{fig.interpolation}, we get some new colors, such as light green, yellow, magenta, dark green, purple, bright green and orange.

\section{More Scene Text Editing Results}
Our method performs well when editing text content on real-world data and avoids the source text shadows, as mentioned in Section 4.3 of the main body.
Due to paper length limitations, we show here more scene text editing results. 
Figure \ref{fig:real_scene} presents string-level qualitative samples, where our method edits the text content while maintaining the original text style and background texture, and the generated images have realistic appearance.
